# Supplementary material for: AF2-Mutation: Adversarial Sequence Mutations against AlphaFold2 on Protein Tertiary Structure Prediction
Source: arXiv:2305.08929 source file (2023-05-15)
Supplement: Supplementary file 1 [file appendix.tex]

\section{Supplementary Material}
\label{sec:appendix}

\begin{figure}[!t]
  \begin{center}
\includegraphics[width=0.9\linewidth]{figs/rep_res.png}
  \end{center}
\caption{The results of the experiments are as follows: (a) The figure illustrates the lDDT difference between the native structure and the adversarial structure, as well as the difference before and after re-alignment. (b) The figure displays the relationship between the plDDT and lDDT. (c) The figure compares the proposed replacement attack method with the random attack, and also shows the distribution of these two results.}
\label{fig:rep_res_fig}
\end{figure}

More details about the results of the CASP14 are listed in the appendix. Figure \ref{fig:rep_res_fig}(a) shows the results of the difference of lDDT between the original lDDT and the adversarial one. The original lDDT is calculated between the native structure and the structure predicted by AlphaFold2. And the adversarial lDDT is computed between the native structure and the adversarial structure predicted by AlphaFold2. The MSA is aligned again when the adversarial structure is predicted, and the final results are shown in Figure~\ref{fig:rep_res_fig}(a).
As shown in Figure~\ref{fig:rep_res_fig}(c), the plDDT is closely related to the lDDT, with a correlation coefficient of 0.66.
And it is clearly shown in Figure~\ref{fig:rep_res_fig}(c) that although not all the sequences in the CASP14 can be attacked successfully, the proposed attack method always outperforms the random one.
